# Supplementary material for: Out-of-Distribution Segmentation in Autonomous Driving: Problems and State of the Art
Source: arXiv:2503.08695 source file (2025-04-05)
Supplement: Supplementary file 1 [file X_suppl.tex]

\clearpage
\setcounter{page}{1}
\maketitlesupplementary

\section{Additional Analysis}
\label{sec:rationale}
